# Supplementary material for: DiffusionLane: Diffusion Model for Lane Detection
Source: arXiv:2510.22236 source file (2025-10-25)
Supplement: Supplementary file 1 [file train.tex]

\small
\caption{\small \ours Training 
}
\label{alg:train}
\algcomment{\fontsize{7.2pt}{0em}\selectfont \texttt{alpha\_cumprod(t)}: cumulative product of $\alpha_i$, \ie, $\prod_{i=1}^t \alpha_i$
}
\definecolor{codeblue}{rgb}{0.25,0.5,0.5}
\definecolor{codegreen}{rgb}{0,0.6,0}
\definecolor{codekw}{RGB}{207,33,46}
\lstset{
  backgroundcolor=\color{white},
  basicstyle=\fontsize{7.5pt}{7.5pt}\ttfamily\selectfont,
  columns=fullflexible,
  breaklines=true,
  captionpos=b,
  commentstyle=\fontsize{7.5pt}{7.5pt}\color{codegreen},
  keywordstyle=\fontsize{7.5pt}{7.5pt}\color{codekw},
  escapechar={|}, 
}
\begin{lstlisting}[language=python]
def train_loss(images, gt_boxes):
  """
  images: [B, H, W, 3]
  gt_boxes: [B, *, 4]
  # B: batch
  # N: number of proposal boxes
  """
  
  # Encode image features
  feats = image_encoder(images)
  
  # Pad gt_boxes to N
  pb = pad_boxes(gt_boxes) # padded boxes: [B, N, 4]

  # Signal scaling
  pb = (pb * 2 - 1) * scale  

  # Corrupt gt_boxes
  t = randint(0, T)|~~~~~~~~~~~|# time step
  eps = normal(mean=0, std=1)  # noise: [B, N, 4]
  pb_crpt = sqrt(|~~~~|alpha_cumprod(t)) * pb + 
              |~|sqrt(1 - alpha_cumprod(t)) * eps

  # Predict
  pb_pred = detection_decoder(pb_crpt, feats, t)

  # Set prediction loss
  loss = set_prediction_loss(pb_pred, gt_boxes)
  
  return loss
\end{lstlisting}
